# Supplementary material for: Experimental measurement-device-independent quantum digital signatures over a metropolitan network
Source: arXiv:1703.01021 ancillary file (2017-03-07)
Supplement: Supplementary file 1 [file Sm-MDIQDS_0227.pdf]

# Supplemental Material: Experimental measurement-device-independent quantum digital signatures over a metropolitan network

Hua-Lei Yin,[1,2] Wei-Long Wang,[3] Yan-Lin Tang,[1,2] Qi Zhao,[4] Hui Liu,[1,2] Xiang-Xiang Sun,[1,2] Wei-Jun Zhang,[5] Hao Li,[5] Ittoop Vergheese Puthoor,[6] Li-Xing You,[5] Erika Andersson,[6] Zhen Wang,[5] Yang Liu,[1,2] Xiao Jiang,[1,2] Xiongfeng Ma,[4,2] Qiang Zhang,[1,2] Marcos Curty,[3] Teng-Yun Chen,[1,2] and Jian-Wei Pan[1,2]

*[1]Hefei National Laboratory for Physical Sciences at Microscale and Department of Modern Physics, University of Science and Technology of China, Hefei, Anhui 230026, China*
*[2]CAS Center for Excellence and Synergetic Innovation Center in Quantum Information and Quantum Physics, University of Science and Technology of China, Hefei, Anhui 230026, China*
*[3]EI Telecomunicación, Department of Signal Theory and Communications, University of Vigo, Vigo E-36310, Spain*
*[4]Center for Quantum Information, Institute for Interdisciplinary Information Sciences, Tsinghua University, Beijing, 100084, China*
*[5]State Key Laboratory of Functional Materials for Informatics, Shanghai Institute of Microsystem and Information Technology, Chinese Academy of Sciences, Shanghai 200050, China*
*[6]SUPA, Institute of Photonics and Quantum Sciences, Heriot-Watt University, Edinburgh EH14 4AS, United Kingdom*

## I. PROTOCOL

Here, we describe the complete measurement-device-independent quantum digital signature (MDI-QDS) protocol in detail. The basic setup is illustrated in Fig. 1. The MDI-QDS scheme consists of two stages: the distribution stage, and the messaging stage. Also, it requires that Bob and Charlie previously share a secret key. In our experiment this is achieved by means of measurement-device-independent quantum key distribution (MDI-QKD).

### A. MDI-QKD protocol

Below we present the different steps of the MDI-QKD protocol which is implemented between Bob and Charlie to distribute a secret key [1].

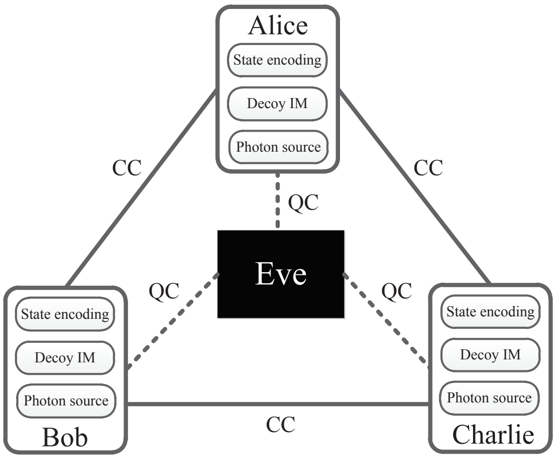


FIG. 1: Schematic diagram of the MDI-QDS setup. The channels between Alice-Eve, Bob-Eve, and Charlie-Eve are quantum channels (QC); they are denoted with dashed lines. Alice-Bob, Alice-Charlie and Bob-Charlie are also connected through authenticated classical channels (CC); these channels are represented with solid lines. The MDI-QDS protocol requires that Bob and Charlie previously share a secret key. For this, they implement a MDI-QKD protocol in which Eve acts as a relay. Each of Alice, Bob and Charlie has one laser source that generates phase-randomised weak coherent pulses which encode different BB84 states by means of a state encoding setup. Also, they generate decoy states with an intensity modulator. This modulator is denoted as Decoy IM in the figure. Eve is supposed to perform a Bell state measurement on the incoming signals. See the main text for further details.

1. *State preparation:* The first two steps of the protocol are repeated $N$ times. In every round, each of Bob and Charlie generates a phase-randomised weak coherent pulse with a randomly selected intensity $\gamma \in \{\mu,\ \nu\ ,0\}$, which encodes a random bit $r \in \{0,\ 1\}$ in a basis $\alpha \in \{Z,\ X\}$ also selected at random. Then they send these pulses to Eve via the quantum channels.

2. *Measurement:* If Eve is honest, she performs a Bell state measurement (BSM) on the signals received from Bob and Charlie. In any case, she announces through a public channel whether or not her measurement is successful, together with the Bell state obtained in case of success.

3. *Sifting:* Once the $N$ rounds of quantum transmission and measurement have finished, Bob and Charlie communicate to each other through an authenticated channel their intensity and basis settings for the successful BSM results. Let $Z_k^{b,c}$ ($X_k^{b,c}$) be the sets that identify those signals where Eve declares the Bell state $k$ and Bob and Charlie select the intensities $b$ and $c$ and the basis Z (X), respectively. If the sifting conditions $|Z_k^{b,c}| \geq N_k^{b,c}$ and $|X_k^{b,c}| \geq M_k^{b,c}$ are satisfied for all $b, c, k$, where $N_k^{b,c}$ and $M_k^{b,c}$ denote some pre-established threshold values, then Bob and Charlie randomly post-select $N_k^{b,c}$ ($M_k^{b,c}$) events from $Z_k^{b,c}$ ($X_k^{b,c}$) to be used in the following steps of the protocol. We will denote such post-selected sets as $\hat{Z}_k^{b,c}$ and $\hat{X}_k^{b,c}$, respectively. That is, $|\hat{Z}_k^{b,c}| = N_k^{b,c}$ and $|\hat{X}_k^{b,c}| = M_k^{b,c}$ for all $b, c, k$. Also, depending on the Bell states announced by Eve, Charlie flips part of his bits to match with those of Bob [2]. If the sifting conditions are not satisfied, the protocol aborts.

4. *Parameter estimation:* Bob and Charlie form the code bit strings $z_k^{b,c}$ and $z_k^{\prime b,c}$, respectively, by randomly choosing $n_k^{b,c}$ bits from $\hat{Z}_k^{b,c}$. The remaining bits of $\hat{Z}_k^{b,c}$, which we denote by $R_k^{b,c}$, are used to compute the error rate $E_k^{b,c}$ and then they are discarded. Only if $E_k^{b,c} \leq E_{\rm tol}$, where $E_{\rm tol}$ is a pre-fixed threshold value, Bob and Charlie use the sets $\hat{Z}_k^{b,c}$ and $\hat{X}_k^{b,c}$ to estimate the following three parameters: $n_{k,0}^{b,c}$ ($n_{k,1}^{b,c}$), which is a lower bound for the number of bits in $z_k^{b,c}$ where Bob (Bob and Charlie) sent a vacuum (single-photon) state, and $e_{k,1}^{b,c}$, which is an upper bound for the single-photon phase error rate in $z_k^{b,c}$. If $E_k^{b,c} > E_{\rm tol}$ for all $k$, the protocol aborts.

5. *Error correction and privacy amplification:* For each intensity setting combination $\{b, c\}$, if the data corresponding to the Bell state $k$ passes the parameter estimation step, then Charlie obtains an estimate of $z_k^{b,c}$, which we shall denote by $\hat{z}_k^{b,c}$, by using an error correction scheme. This scheme requires that Bob sends Charlie ${\rm leak}_{{\rm EC},k}^{b,c}$ bits of error correction information. Afterward, Bob and Charlie implement an error verification protocol to confirm that $z_k^{b,c}$ and $\hat{z}_k^{b,c}$ are indeed equal except for a minuscule probability $\epsilon_{\rm cor}^{b,c}$. For this, Bob randomly selects a universal$_2$ hash function *hash* and sends it to Charlie together with the hash value $hash(z_k^{b,c})$. The protocol aborts if $hash(\hat{z}_k^{b,c}) \neq hash(z_k^{b,c})$, $\forall k$. Otherwise, Bob and Charlie perform privacy amplification to extract two shorter bit strings $S_k^{b,c}$ and $\hat{S}_k^{b,c}$ of length $\ell_k^{b,c}$ from $z_k^{b,c}$ and $\hat{z}_k^{b,c}$, respectively. They form the final secret key $S_{\rm B}$ and $S_{\rm C}$ by concatenating the bit strings $S_k^{b,c}$ and $\hat{S}_k^{b,c}$, respectively. That is, the length of the secret key is $|S_{\rm B}| = |S_{\rm C}| = \sum\limits_{b,c\in\{0,\nu,\mu\}} \sum_k \ell_k^{b,c}$.

### B. MDI-QDS scheme

We now describe the procedure for signing a binary message. As already mentioned above, the MDI-QDS scheme consists of the distribution and the messaging stages. See [3] for more details. Below we assume that Bob and Charlie have already performed the MDI-QKD scheme and they share a secret key.

#### *1. Distribution stage*

For each possible bit message $m \in \{0, 1\}$, Alice performs a measurement-device-independent key generation protocol (MDI-KGP) with Bob and Charlie. As discussed in the main text, this protocol provides Alice with different $L$-bit strings $A_m^{\rm B}$ ($A_m^{\rm C}$), which are correlated with the ones that are obtained by Bob (Charlie). We denote Bob's (Charlie's) $L$-bit strings by $K_m^{\rm B}$ ($K_m^{\rm C}$).

For this, the MDI-KGP builds on the MDI-QKD protocol described in the previous section but with a few modifications. In particular, let us take the MDI-KGP between Alice and Bob as an example, the MDI-KGP between Alice and Charlie is analogous. To generate the correlated bit strings $A_m^{\rm B}$ and $K_m^{\rm B}$ with $m \in \{0, 1\}$, Alice and Bob only perform the first four steps of the MDI-QKD protocol. That is, they do not implement the classical post-processing steps of error correction and privacy amplification. Also, for simplicity, we will consider that they use only the data associated with a projection onto one particular Bell state $k$ and discard the rest. In addition, Alice and Bob modify the parameter estimation step of the MDI-QKD scheme as

follows. They randomly distribute the bits from $\hat{Z}_k^{\mu,\mu}$ into two sets of equal size, which we shall denote by $\hat{Z}_{k,m}^{\mu,\mu}$ with $m \in \{0,1\}$. Then, they both respectively obtain $A_m^{\mathrm{B}}$ and $K_m^{\mathrm{B}}$ by simply selecting at random $L$ bits from each of these sets. The remaining bits ($R_{k,m}^{\mu,\mu}$) from $\hat{Z}_{k,m}^{\mu,\mu}$ are used to calculate the bit error rate $E_{k,m}^{\mu,\mu}$. This bit error rate must be below a certain threshold value for all $m$. Otherwise the protocol aborts.

Next, Bob and Charlie symmetrize the resulting bit strings $K_m^{\mathrm{B}}$ and $K_m^{\mathrm{C}}$. This is achieved by each of them initially selecting half of the bits of their respective bit strings at random, and then sending these bits (as well as the corresponding bit positions) through their secure channel. That is, say Bob randomly chooses $L/2$ bits from $K_m^{\mathrm{B}}$ and sends them to Charlie (together with the information of their positions in $K_m^{\mathrm{B}}$) encrypted with the one-time pad. Likewise, Charlie does the same with $K_m^{\mathrm{C}}$. We will denote the symmetrized $L$-bit strings of Bob and Charlie by $S_m^{\mathrm{B}}$ and $S_m^{\mathrm{C}}$, respectively. That is, $S_m^{\mathrm{B}}$ ($S_m^{\mathrm{C}}$) is composed by the part of $K_m^{\mathrm{B}}$ ($K_m^{\mathrm{C}}$) that Bob (Charlie) decides to keep, which we shall denote by $K_{\mathrm{keep},m}^{\mathrm{B}}$ ($K_{\mathrm{keep},m}^{\mathrm{C}}$), and the part of $K_m^{\mathrm{C}}$ ($K_m^{\mathrm{B}}$) received from Charlie (Bob), which we shall denote by $K_{\mathrm{forward},m}^{\mathrm{C}}$ ($K_{\mathrm{forward},m}^{\mathrm{B}}$).

Finally, Bob estimates the quantities $n_{m,0}$, $n_{m,1}$ and $e_{m,1}$ for the bit strings $K_{\mathrm{keep},m}^{\mathrm{B}}$, where $n_{m,0}$ ($n_{m,1}$) represents a lower bound for the number of bits in $K_{\mathrm{keep},m}^{\mathrm{B}}$ where Bob (Alice and Bob) sent a vacuum (single-photon) state, and $e_{m,1}$ is an upper bound for the single-photon phase error rate. Likewise, Charlie does the same with $K_{\mathrm{keep},m}^{\mathrm{C}}$.

### 2. *Messaging stage*

To sign a binary message $m$, Alice sends $(m, \mathrm{Sig}_m)$ to the desired recipient (say for instance Bob), where $\mathrm{Sig}_m = (A_m^{\mathrm{B}}, A_m^{\mathrm{C}})$ is the signature of $m$. Then, Bob records the number of mismatches between $\mathrm{Sig}_m$ and $S_m^{\mathrm{B}}$ by separately comparing $A_m^{\mathrm{B}}$ with the part, $K_{\mathrm{keep},m}^{\mathrm{B}}$, of $S_m^{\mathrm{B}}$ received from Alice and $A_m^{\mathrm{C}}$ with the part, $K_{\mathrm{forward},m}^{\mathrm{C}}$, of $S_m^{\mathrm{B}}$ received from Charlie. If there are fewer than $s_a(L/2)$ mismatches in both cases, where $s_a < 1/2$ is a small threshold value that is determined by certain experimental parameters which depend on the desired security level of the protocol, Bob then accepts the message as coming from Alice.

If Bob wants to prove Charlie that he received the message $m$ from Alice, he forwards him $(m, \mathrm{Sig}_m)$. Then, Charlie checks the mismatches between $\mathrm{Sig}_m$ and $S_m^{\mathrm{C}}$ in a similar way like Bob, and accepts $m$ if the number of mismatches is less than $s_v(L/2)$, where $s_v$ is another threshold value which satisfies $0 < s_a < s_v < 1/2$.

## II. SECRET KEY DISTILLATION

The symmetrization step of the MDI-QDS protocol requires that Bob and Charlie interchange half of their bits (together with the information of the positions of the bits interchanged) in full secrecy. This means, in particular, that they need a secret key of length at least $6L$ to be used with the one-time pad. This is so because, as we saw in the main text, we need $3L/2$ secret bits for each $K_m^{\mathrm{B}}$ (or $K_m^{\mathrm{C}}$) with $m \in \{0,1\}$.

To determine the secret key length of the MDI-QKD link between Bob and Charlie we follow the finite-key analysis provided in [1]. In our experiment, Eve's BSM performs projections only onto one single Bell state $k$, so for simplicity below we remove the label $k$ from all the parameters. Also, as already mentioned in the previous section, note that Bob and Charlie distill secret key from all the events where both of them select the Z basis and Eve declares a successful result, *i.e.*, independently of the particular intensity setting selected. Thus, according to [1] we have that the length $\ell$ of the secret bit strings $S_{\mathrm{B}}$ and $S_{\mathrm{C}}$ is given by

$$\ell \geq \sum_{b,c\in\{0,\,\nu,\,\mu\}} \ell^{b,c}, \tag{1}$$

with

$$\ell^{b,c} = \max\left\{ n_0^{b,c} + n_1^{b,c}\left[1 - h\left(e_1^{b,c}\right)\right] - \mathrm{leak}_{\mathrm{EC}}^{b,c} - \log_2\frac{8}{\epsilon_{\mathrm{cor}}^{b,c}} - 2\log_2\frac{2}{\varepsilon'^{b,c}\hat{\varepsilon}^{b,c}} - 2\log_2\frac{1}{2\varepsilon_{\mathrm{PA}}^{b,c}}, 0\right\}. \tag{2}$$

The definition of the different parameters is given in the main text. We include it again here for completeness. In particular, we have that $h(x) = -x\log_2(x) - (1-x)\log_2(1-x)$ is the binary Shannon entropy function, $\epsilon_{\mathrm{cor}} = \sum_{b,c}\epsilon_{\mathrm{cor}}^{b,c}$ is the correctness parameter with $\epsilon_{\mathrm{cor}}^{b,c}$ being the failure probability of the error verification step which is applied to the bit strings $z^{b,c}$ and $\hat{z}^{b,c}$, and $\epsilon_{\mathrm{sec}} = \sum_{b,c}\epsilon_{\mathrm{sec}}^{b,c}$ is the secrecy parameter, with $\epsilon_{\mathrm{sec}}^{b,c} = 2\left(\varepsilon'^{b,c} + 2\varepsilon_e^{b,c} + \hat{\varepsilon}^{b,c}\right) + \varepsilon_\beta^{b,c} + \varepsilon_0^{b,c} + \varepsilon_1^{b,c} + \varepsilon_{\mathrm{PA}}^{b,c}$. The parameters $\varepsilon_0^{b,c}$, $\varepsilon_1^{b,c}$ and $\varepsilon_e^{b,c}$ denote the failure probability associated with the estimation of $n_0^{b,c}$, $n_1^{b,c}$ and $e_1^{b,c}$, respectively, and $\varepsilon_{\mathrm{PA}}^{bc}$ represents the failure probability of the privacy amplification step.

To estimate the parameters $n_0^{b,c}$, $n_1^{b,c}$ and $e_1^{b,c}$ we follow the method used in [4]. In particular, let us denote the data that we observe in the experiment as follows. $N_{bc}^{\alpha\beta}$ is the total number of pulses prepared by Bob and Charlie by using the bases $\alpha$ and $\beta$ and the intensities $b$ and $c$, respectively, with $\alpha, \beta \in \{Z, X\}$ and $b, c \in \{0,\ \nu,\ \mu\}$. $D_{bc}^{\alpha\beta}$ is the total number of successful BSM events reported by Eve given that Bob and Charlie used the bases $\alpha$ and $\beta$ and the intensities $b$ and $c$, respectively. $E_{bc}^{\alpha\beta}$ is the number of errors in $D_{bc}^{\alpha\beta}$.

Then, after applying the sifting step of the protocol, we have that only the data where Bob and Charlie use the same basis remains. Importantly, however, the data associated with those events where Bob or Charlie (or both of them together) send a vacuum state does not need to be distinguished by the encoding basis but it can be assigned to any basis. This means, in particular, that Bob and Charlie can use data from mismatched basis events where they send vacuum states to obtain a tighter estimation of the parameters $n_0^{b,c}$, $n_1^{b,c}$ and $e_1^{b,c}$ in the finite key regime. For instance, they can redefine the observed data in the $Z$ and $X$ bases as follows. See [4] for further details.

$$
\begin{array}{lllll}
M_{\mu\mu}^{\rm Z} = M_{\mu\mu}^{\rm ZZ}, & M_{\mu 0}^{\rm Z} = M_{\mu 0}^{\rm ZZ}, & M_{00}^{\rm Z} = M_{00}^{\rm ZZ}, & M_{\nu\nu}^{\rm X} = M_{\nu\nu}^{\rm XX} & M_{0\nu}^{\rm X} = M_{0\nu}^{\rm XX} + M_{0\nu}^{\rm ZX}, \\
M_{\mu\nu}^{\rm Z} = M_{\mu\nu}^{\rm ZZ}, & M_{0\mu}^{\rm Z} = M_{0\mu}^{\rm ZZ}, & M_{\mu\mu}^{\rm X} = M_{\mu\mu}^{\rm XX}, & M_{\mu 0}^{\rm X} = M_{\mu 0}^{\rm XX} + M_{\mu 0}^{\rm XZ}, & M_{00}^{\rm X} = M_{00}^{\rm XX} + M_{00}^{\rm ZX} + M_{00}^{\rm XZ}, \\
M_{\nu\mu}^{\rm Z} = M_{\nu\mu}^{\rm ZZ}, & M_{\nu 0}^{\rm Z} = M_{\nu 0}^{\rm ZZ}, & M_{\mu\nu}^{\rm X} = M_{\mu\nu}^{\rm XX}, & M_{0\mu}^{\rm X} = M_{0\mu}^{\rm XX} + M_{0\mu}^{\rm ZX}, & \\
M_{\nu\nu}^{\rm Z} = M_{\nu\nu}^{\rm ZZ}, & M_{0\nu}^{\rm Z} = M_{0\nu}^{\rm ZZ}, & M_{\nu\mu}^{\rm X} = M_{\nu\mu}^{\rm XX}, & M_{\nu 0}^{\rm X} = M_{\nu 0}^{\rm XX} + M_{\nu 0}^{\rm XZ}, &
\end{array}
\tag{3}
$$

where $M \in \{N, D, E\}$, *i.e.*, the equations above are applied to $N_{bc}^{\alpha\beta}$, $D_{bc}^{\alpha\beta}$ and $E_{bc}^{\alpha\beta}$. Afterward, Bob and Charlie use a standard estimation procedure [1] on the redefined parameters to determine $n_0^{b,c}$, $n_1^{b,c}$ and $e_1^{b,c}$.

## III. SECURITY PARAMETERS OF MDI-QDS

Since the secret key obtained from the MDI-QKD protocol is used to encrypt the information interchanged between Bob and Charlie in the key symmetrization step of the MDI-QDS scheme, the security parameters of both protocols should be of the same order of magnitude in order to optimize the security level of the experiment.

Next, we describe how to calculate the security parameters of the MDI-QDS protocol. The analysis is based on the results introduced in [3]. In particular, we have that the robustness of the protocol, *i.e.*, the probability of an honest run aborting, depends mainly on the parameter $s_a$ which determines if Bob accepts a message received from Alice. For MDI-QDS, we choose $s_a > \bar{E}$, where $\bar{E} = \max\{E_m^{\rm B}, E_m^{\rm C}\}$ and

$$
E_m^{\rm B} \geq E_{AB,m}^{\mu\mu} + g\left(\frac{L}{2},\, R_{AB,m}^{\mu\mu},\, \varepsilon_{\rm PE}\right), \tag{4}
$$

with

$$
g\left(\frac{L}{2}, R_{AB,m}^{\mu\mu}, \varepsilon_{\rm PE}\right) = \sqrt{\frac{\left(R_{AB,m}^{\mu\mu} + L/2\right)\left(R_{AB,m}^{\mu\mu} + 1\right)\ln\left(\varepsilon_{\rm PE}{}^{-1}\right)}{\left(R_{AB,m}^{\mu\mu}\right)^2 L/2}}. \tag{5}
$$

The parameters $E_{AB,m}^{\mu\mu}$ and $R_{AB,m}^{\mu\mu}$ refer to the quantities $E_{k,m}^{\mu\mu}$ and $R_{k,m}^{\mu\mu}$ introduced in Sec. I B for the MDI-KGP between Alice and Bob. Here, we have removed the subscript $k$ because, as already mentioned, in our experiment Eve performs projections onto only one single Bell state, and we have added the subscript AB to emphasise that we refer to the link Alice-Bob. Eq. (4) represents an upper bound on the error rate between Bob's bit string $K_{{\rm keep},m}^{\rm B}$ and the corresponding bits from Alice's bit string $A_m^{\rm B}$, which is correct except for a failure probability $\varepsilon_{\rm PE}$. The parameter $E_m^{\rm C}$ is defined in a similar way but now for the link Alice-Charlie.

Then, it can be shown that the robustness of the MDI-QDS protocol is given by

$$
\varepsilon_{\rm rob} \leq 2\varepsilon_{\rm PE}, \tag{6}
$$

which is the probability that either $\bar{E}_{AB,m}^{\mu\mu}$ or $\bar{E}_{AC,m}^{\mu\mu}$ is not an upper bound for $E_{AB,m}^{\mu\mu}$ or $E_{AC,m}^{\mu\mu}$, respectively.

On the other hand, it turns out that the probability that Alice can successfully repudiate the signature of a message satisfies

$$
\varepsilon_{\rm rep} \leq 2\exp\left[-\frac{1}{4}(s_v - s_a)^2 L\right] + \epsilon_{\rm QKD}, \tag{7}
$$

where $\epsilon_{\rm QKD} = \epsilon_{\rm cor} + \epsilon_{\rm sec}$ is the probability that the secret key shared between Bob and Charlie by means of MDI-QKD is insecure.

TABLE 1: List of the experimental results in MDI-KGP between Bob and Alice.

| $B-E-A$ | Number of detection events | | | Number of errors | | | Total number of pulses | | |
|---|---|---|---|---|---|---|---|---|---|
| | $0-Z$ | $\nu-Z$ | $\mu-Z$ | $0-Z$ | $\nu-Z$ | $\mu-Z$ | $0-Z$ | $\nu-Z$ | $\mu-Z$ |
| $0-Z$ | 5 | 2281 | 9410 | 0 | 1151 | 4678 | 3.48E+10 | 9.46E+10 | 1.13E+11 |
| $\nu-Z$ | 6102 | 1749934 | 6900463 | 3097 | 11321 | 23079 | 9.46E+10 | 2.56E+11 | 3.04E+11 |
| $\mu-Z$ | 25327 | 6637000 | 25920132 | 12597 | 37586 | 57933 | 1.13E+11 | 3.04E+11 | 3.61E+11 |
| | $0-X$ | $\nu-X$ | $\mu-X$ | $0-X$ | $\nu-X$ | $\mu-X$ | $0-X$ | $\nu-X$ | $\mu-X$ |
| $0-X$ | 3 | 221587 | 0 | 0 | 109383 | 0 | 3.48E+10 | 1.62E+11 | 0 |
| $\nu-X$ | 1567663 | 13559453 | 0 | 792879 | 4495014 | 0 | 1.62E+11 | 7.50E+11 | 0 |
| $\mu-X$ | 0 | 0 | 0 | 0 | 0 | 0 | 0 | 0 | 0 |
| | $0-Z$ | $\nu-Z$ | $\mu-Z$ | $0-Z$ | $\nu-Z$ | $\mu-Z$ | $0-Z$ | $\nu-Z$ | $\mu-Z$ |
| $0-X$ | 8 | 2109 | 9926 | 0 | 1023 | 5094 | 3.58E+10 | 8.91E+10 | 1.17E+11 |
| $\nu-X$ | 1559324 | 7353412 | 16949068 | 752481 | 3699305 | 8601812 | 1.61E+11 | 4.43E+11 | 5.16E+11 |
| $\mu-X$ | 0 | 0 | 0 | 0 | 0 | 0 | 0 | 0 | 0 |
| | $0-X$ | $\nu-X$ | $\mu-X$ | $0-X$ | $\nu-X$ | $\mu-X$ | $0-X$ | $\nu-X$ | $\mu-X$ |
| $0-Z$ | 10 | 224153 | 0 | 1 | 108354 | 0 | 3.32E+10 | 1.63E+11 | 0 |
| $\nu-Z$ | 6342 | 3600069 | 0 | 3150 | 1794446 | 0 | 9.91E+10 | 4.33E+11 | 0 |
| $\mu-Z$ | 24754 | 12375438 | 0 | 12589 | 6171201 | 0 | 1.10E+10 | 5.23E+11 | 0 |

TABLE 2: List of the experimental results in MDI-KGP between Alice and Charlie.

| $A-E-C$ | Number of detection events | | | Number of errors | | | Total number of pulses | | |
|---|---|---|---|---|---|---|---|---|---|
| | $0-Z$ | $\nu-Z$ | $\mu-Z$ | $0-Z$ | $\nu-Z$ | $\mu-Z$ | $0-Z$ | $\nu-Z$ | $\mu-Z$ |
| $0-Z$ | 56 | 2732 | 11538 | 33 | 1358 | 5889 | 7.12E+10 | 1.93E+11 | 2.30E+11 |
| $\nu-Z$ | 2676 | 1901132 | 7467976 | 1396 | 7043 | 19402 | 1.93E+11 | 5.22E+11 | 6.21E+11 |
| $\mu-Z$ | 11164 | 7547507 | 29400832 | 15521 | 18995 | 37340 | 2.30E+11 | 6.21E+11 | 7.37E+11 |
| | $0-X$ | $\nu-X$ | $\mu-X$ | $0-X$ | $\nu-X$ | $\mu-X$ | $0-X$ | $\nu-X$ | $\mu-X$ |
| $0-X$ | 53 | 934208 | 0 | 29 | 468323 | 0 | 7.12E+10 | 3.30E+11 | 0 |
| $\nu-X$ | 468796 | 12232268 | 0 | 233884 | 3784406 | 0 | 3.30E+11 | 1.53E+12 | 0 |
| $\mu-X$ | 0 | 0 | 0 | 0 | 0 | 0 | 0 | 0 | 0 |
| | $0-Z$ | $\nu-Z$ | $\mu-Z$ | $0-Z$ | $\nu-Z$ | $\mu-Z$ | $0-Z$ | $\nu-Z$ | $\mu-Z$ |
| $0-X$ | 71 | 2644 | 11841 | 32 | 1303 | 6184 | 7.32E+10 | 1.82E+11 | 2.40E+11 |
| $\nu-X$ | 459779 | 4574929 | 14265714 | 226537 | 2306807 | 7214626 | 3.28E+11 | 9.05E+11 | 1.05E+12 |
| $\mu-X$ | 0 | 0 | 0 | 0 | 0 | 0 | 0 | 0 | 0 |
| | $0-X$ | $\nu-X$ | $\mu-X$ | $0-X$ | $\nu-X$ | $\mu-X$ | $0-X$ | $\nu-X$ | $\mu-X$ |
| $0-Z$ | 55 | 894712 | 0 | 38 | 435637 | 0 | 6.79E+10 | 3.34E+11 | 0 |
| $\nu-Z$ | 2634 | 5801820 | 0 | 1306 | 2909919 | 0 | 2.02E+11 | 8.85E+11 | 0 |
| $\mu-Z$ | 10616 | 16239773 | 0 | 5316 | 7809247 | 0 | 2.25E+11 | 1.07E+12 | 0 |

In our simulations, we set the threshold parameters $s_a$ and $s_v$ as $s_a = \bar{E} + \frac{p_E - \bar{E}}{50}$ and $s_v = \bar{E} + \frac{49(p_E - \bar{E})}{50}$, respectively. In general, the parameter $p_{\rm E}$ represents the minimum rate at which a potential eavesdropper can make errors when guessing $K^{\rm B}_{{\rm keep},m}$ or $K^{\rm C}_{{\rm keep},m}$. That is, we set $p_{\rm E} := \min\{p^{\rm AB}_{\rm E}, p^{\rm AC}_{\rm E}\}$, where $p^{\rm AB}_{\rm E}$ and $p^{\rm AC}_{\rm E}$ are the rates at which the eavesdropper can make errors in guessing the respective strings $K^{\rm B}_{{\rm keep},m}$ and $K^{\rm C}_{{\rm keep},m}$. This is given by

$$h\left(p^{\rm J}_{\rm E}\right) = c^{\rm J}_{m,0} + c^{\rm J}_{m,1}\left[1 - h\left(e^{\rm J}_{m,1}\right)\right], \tag{8}$$

where $J \in \{AB, AC\}$. Here, $c^{\rm J}_{m,i} := 2n^{\rm J}_{m,i}/L$ and $e^{\rm J}_{m,1}$ refer to the parameters estimated from $K^{\rm B}_{{\rm keep},m}$ and $K^{\rm C}_{{\rm keep},m}$. In our experiment, since we implement the case where Alice sends a signed message to Bob, we can take $p_{\rm E}$ as $p^{\rm AB}_{\rm E}$.

The threshold parameters $s_a$ and $s_v$ have to satisfy the condition $\bar{E} < s_a < s_v < p_E$ [3]. Also, Eq. (7) indicates that the bigger the gap between $s_a$ and $s_v$ is, the smaller would be $\varepsilon_{\rm rep}$. This means that $s_a$ should be chosen close to $\bar{E}$. In the case of $s_v$, however, there is one additional constraint that must be satisfied. It arises from the need that the probability $(p_{\rm r})$ that

TABLE 3: List of the experimental results in the MDI-QKD protocol between Bob and Charlie.

| $B-E-C$ | Number of detection events | | | Number of errors | | | Total number of pulses | | |
|---|---|---|---|---|---|---|---|---|---|
| | $0-Z$ | $\nu-Z$ | $\mu-Z$ | $0-Z$ | $\nu-Z$ | $\mu-Z$ | $0-Z$ | $\nu-Z$ | $\mu-Z$ |
| $0-Z$ | 26 | 3030 | 12044 | 9 | 1577 | 6040 | 3.87E+10 | 1.05E+11 | 1.25E+11 |
| $\nu-Z$ | 7767 | 2270167 | 8869003 | 3864 | 13852 | 27681 | 1.05E+11 | 2.84E+11 | 3.38E+11 |
| $\mu-Z$ | 30578 | 8584134 | 33191574 | 15469 | 46320 | 68734 | 1.25E+11 | 3.38E+11 | 4.01E+11 |
| | $0-X$ | $\nu-X$ | $\mu-X$ | $0-X$ | $\nu-X$ | $\mu-X$ | $0-X$ | $\nu-X$ | $\mu-X$ |
| $0-X$ | 16 | 374541 | 0 | 10 | 189842 | 0 | 3.87E+10 | 1.80E+11 | 0 |
| $\nu-X$ | 1692163 | 16386192 | 0 | 843731 | 5228055 | 0 | 1.80E+11 | 8.34E+11 | 0 |
| $\mu-X$ | 0 | 0 | 0 | 0 | 0 | 0 | 0 | 0 | 0 |
| | $0-Z$ | $\nu-Z$ | $\mu-Z$ | $0-Z$ | $\nu-Z$ | $\mu-Z$ | $0-Z$ | $\nu-Z$ | $\mu-Z$ |
| $0-X$ | 17 | 3055 | 12550 | 10 | 1487 | 6412 | 3.98E+10 | 9.90E+10 | 1.30E+11 |
| $\nu-X$ | 1699809 | 8511993 | 20790027 | 829897 | 4220816 | 10849002 | 1.79E+11 | 4.93E+11 | 5.74E+11 |
| $\mu-X$ | 0 | 0 | 0 | 0 | 0 | 0 | 0 | 0 | 0 |
| | $0-X$ | $\nu-X$ | $\mu-X$ | $0-X$ | $\nu-X$ | $\mu-X$ | $0-X$ | $\nu-X$ | $\mu-X$ |
| $0-Z$ | 26 | 359290 | 0 | 14 | 173852 | 0 | 3.69E+10 | 1.82E+11 | 0 |
| $\nu-Z$ | 7270 | 5072023 | 0 | 3632 | 2560729 | 0 | 1.10E+11 | 4.82E+11 | 0 |
| $\mu-Z$ | 30047 | 16514489 | 0 | 14986 | 8200455 | 0 | 1.22E+11 | 5.82E+11 | 0 |

TABLE 4: List of experimental parameters related to the creation of the signatures $A_m^{\rm B}$, $A_m^{\rm C}$, $K_m^{\rm B}$ and $K_m^{\rm C}$

| | $\lvert\hat{Z}_{k,m}^{\mu,\mu}\rvert$ | $L$ | $\lvert R_{k,m}^{\mu,\mu}\rvert$ | Number of errors | $E_{k,m}^{\mu,\mu}$ |
|---|---|---|---|---|---|
| $A_0^B-K_0^B$ | 12960066 | 787468 | 12172598 | 26880 | 0.219% |
| $A_1^B-K_1^B$ | 12960066 | 787468 | 12172598 | 27479 | 0.225% |
| $A_0^C-K_0^C$ | 14700416 | 787468 | 13912947 | 17786 | 0.127% |
| $A_1^C-K_1^C$ | 14700416 | 787468 | 13912947 | 17573 | 0.126% |

Bob makes fewer than $s_v L/2$ errors when guessing $K_{{\rm keep},m}^{\rm C}$ has to be smaller than a security parameter $f$, which protects the protocol against forging. More precisely, according to [3] we have that the probability $p_{\rm r}$ is upper bounded by

$$\langle p_{\rm r}\rangle \leq \sum_{i=0}^{s_v L/2}\binom{L/2}{i}2^{-H_{\rm min}^{\epsilon}\left(K_{{\rm keep},m}^{\rm C}|B\right)}+\varepsilon_{\rm H}, \tag{9}$$

where

$$H_{\rm min}^{\epsilon}\left(K_{{\rm keep},m}^{\rm C}|B\right)\approx n_{m,0}+n_{m,1}\left[1-h\left(e_{m,1}\right)\right], \tag{10}$$

is Bob's smooth min-entropy about Charlie's bit string $K_{{\rm keep},m}^{\rm C}$, and $\varepsilon_{\rm H}$ is the failure probability related to the estimation of this smooth min-entropy. Eq. (9) can be further upper bounded as follows,

$$\begin{aligned}\langle p_{\rm r}\rangle &\leq \sum_{i=0}^{s_v L/2}\tbinom{L/2}{i}2^{-\{n_{m,0}+n_{m,1}[1-h(e_{m,1})]\}}+\varepsilon_{\rm H}=\sum_{i=0}^{s_v L/2}\tbinom{L/2}{i}2^{-\frac{L}{2}h(p_E)}+\varepsilon_{\rm H}\\ &\leq \sum_{i=0}^{s_v L/2}\tbinom{L/2}{s_v L/2}2^{-\frac{L}{2}h(p_E)}+\varepsilon_{\rm H}\leq \sum_{i=0}^{s_v L/2}2^{\frac{L}{2}h(s_v)}2^{-\frac{L}{2}h(p_E)}+\varepsilon_{\rm H}=\left(\tfrac{s_v L}{2}+1\right)2^{-\frac{L}{2}[h(p_E)-h(s_v)]}+\varepsilon_{\rm H}.\end{aligned} \tag{11}$$

The first inequality is due to Eq. (10); in the second one we use Eq. (8); in the third one we use a property of the binomial coefficient together with the fact that $s_v<1/2$; and in the fourth inequality we use $\binom{N}{k}\leq 2^{Nh\left(\frac{k}{N}\right)}$.

This means, in particular, that if $s_v$ is chosen smaller than (but very close to) $p_E$ such that $\left(\frac{s_v L}{2}+1\right)2^{-\frac{L}{2}[h(p_E)-h(s_v)]}$ is relatively small in comparison to $\varepsilon_{\rm H}$, and $f$ is chosen larger than Eq. (11), the resulting value of $\varepsilon_{\rm rep}$ decreases. This can be achieved, for instance, by setting $s_a=\bar{E}+\frac{p_E-\bar{E}}{50}$ and $s_v=\bar{E}+\frac{49\left(p_E-\bar{E}\right)}{50}$, which provide better results than those reported in [3].

Finally, we have that the probability that Bob can successfully forge a message $m$ is given by

$$\varepsilon_{\rm for} \leq p_{\rm F} + f + \varepsilon_{\rm PE} + \varepsilon_{m,0} + \varepsilon_{m,1} + \varepsilon_{m,e}, \tag{12}$$

where

$$p_{\rm F} := \frac{1}{f}\left(2^{-\frac{L}{2}\{c_{m,0}+c_{m,1}[1-h(e_{m,1})]-h(s_v)\}} + \varepsilon_{\rm H}\right), \tag{13}$$

and $\varepsilon_{m,0},\ \varepsilon_{m,1},\ \varepsilon_{m,e}$ are the failure probabilities related to the estimation of $n_{m,0},\ n_{m,1}\ , e_{m,1}$.

For simulation purposes, we set the security level of the MDI-QKD protocol as $\epsilon_{\rm QKD} = 8 \times 10^{-8}$ and we obtain a final secret key length of $\ell = 4724819$. The threshold parameters of the MDI-QDS scheme take the value $s_a = 0.27\%$ and $s_v = 1.21\%$, and we obtain $\varepsilon_{\rm rob} = 2 \times 10^{-8}$, $\varepsilon_{\rm rep} = 1.51 \times 10^{-7}$ and $\varepsilon_{\rm for} = 9.76 \times 10^{-8}$. That is, we observe an experimental demonstration of the complete MDI-QDS protocol with a total security level of the order of $10^{-7}$.

## IV. EXPERIMENTAL RESULTS

The detailed experimental results for the MDI-KGP and the MDI-QKD protocol are shown in Tables 1, 2 and 3. These tables present the total number of signals sent, the number of detection events and the number of errors for all possible combinations of intensity and basis settings.

Finally, in Table 4 we show the experimental results related to the creation of the signatures $A_m^{\rm B}$, $A_m^{\rm C}$, $K_m^{\rm B}$, and $K_m^{\rm C}$. As already mentioned above, the sets $\hat{Z}_{k,m}^{\mu,\mu}$ with $m \in \{0,1\}$ are obtained by randomly distributing the bits from $\hat{Z}_k^{\mu,\mu}$ into two sets. Then, from each set $\hat{Z}_{k,m}^{\mu,\mu}$ we select $L$ bits at random to form the signatures, while the remaining bits $R_{k,m}^{\mu,\mu}$ from $\hat{Z}_{k,m}^{\mu,\mu}$ are used to estimate the error rate. In Table 4, the column that contains the number of errors refers to the number of error found in $R_{k,m}^{\mu,\mu}$.


[1] M. Curty, F. Xu, W. Cui, C. C. W. Lim, K. Tamaki, and H.-K. Lo, Nature communications **5** (2014).
[2] H.-K. Lo, M. Curty, and B. Qi, Physical Review Letters **108**, 130503 (2012).
[3] I. V. Puthoor, R. Amiri, P. Wallden, M. Curty, and E. Andersson, Physical Review A **94**, 022328 (2016).
[4] Y.-L. Tang, H.-L. Yin, Q. Zhao, H. Liu, X.-X. Sun, M.-Q. Huang, W.-J. Zhang, S.-J. Chen, L. Zhang, L.-X. You, *et al.*, Physical Review X **6**, 011024 (2016).
